# Supplementary material for: Zero-Inflated Bandits
Source: arXiv:2312.15595 source file (2025-01-31)
Supplement: Supplementary file 1 [file 9_additional_literature_review.tex]

\section{Related Works on Zero-Inflated Structures}\label{app_other_ZI_review}

% The Zero-Inflated (ZI) has been noticed for quite a long time, especially in the analysis of counting processes \cite{lambert1992zero,hall2000zero,cheung2002zero}. But most of these studies primarily focus on offline learning scenarios, where the objective is to analyze datasets post-collection, a context significantly different from the online learning challenges presented by bandit problems. In contrast, the ZI bandit is applying the ZI model within the online learning paradigm of bandit algorithms. This shift to an online framework necessitates novel analytical techniques, including the development of specialized concentration inequalities to handle the ZI structure effectively. 
Zero-Inflated (ZI) structures have long been recognized, particularly in the analysis of counting processes \cite{lambert1992zero, hall2000zero, cheung2002zero}. However, most studies focus on offline learning scenarios, where the goal is to analyze datasets post-collection: a context quite different from the online learning challenges presented by bandit problems. In contrast, applying the ZI model within bandit algorithms requires specialized concentration inequalities to handle the ZI structure effectively.

Some online learning literature addresses ZI structures, with zero-inflated online pricing being particularly relevant to our model. For instance, \cite{trovo2018improving} examines dynamic pricing within a multi-armed bandit framework where zero rewards are common. Subsequent studies, such as \cite{bernasconi2022dark, genalti2022dynamic, mussi2022pricing}, explore complex settings in e-commerce and dynamic pricing. However, these models fix the price $a_t$ for each action, corresponding to our non-zero reward component $X_t$, while in our framework, this component is entirely random. This difference allows our method to capture the complexities and uncertainties inherent in real-world applications more comprehensively. Our work extends and generalizes existing models by introducing randomness to the non-zero reward component, offering a broader perspective on handling ZI structures. The resulting algorithm provides theoretical guarantees and focuses on the random nature of non-zero rewards. To the best of our knowledge, this is the first attempt to explore such ZI models.

% On the other hand, there does exist some online learning literature for ZI structure. Specially, the zero-inflated online pricing is closely related to our model. For example, \cite{trovo2018improving} also study dynamic pricing for MAB model, where zero rewards are common. Subsequent literature, including works by \cite{bernasconi2022dark,genalti2022dynamic,mussi2022pricing}, explores complex settings within e-commerce and dynamic pricing.
% The major difference is that for such model, the price $a_t$ for each action, which corresponds to our non-zero reward component, $X_t$, is fixed. In contrast,  this component in our setting is totally be random. This distinction enables our method to more fully capture the complexities and uncertainties inherent in many real-world applications, offering a broader perspective on handling ZI structures. Considering this, our work can be seen as an extension and generalization of the models in such literatures, addressing a wider array of scenarios through the introduction of randomness in the reward's non-zero component. 
% Our contribution is distinguished by its focus on the random nature of the non-zero rewards and the provision of a corresponding algorithm with theoretical guarantees.

% Indeed, To the best of our knowledge, this is the first endeavor to explore the ZI model's within the framework of bandit problems. 
